# Supplementary material for: Selecting the Number of Clusters $K$ with a Stability Trade-off: an Internal Validation Criterion
Source: arXiv:2006.08530 source file (2023-05-16)
Supplement: Supplementary file 1 [file results.tex]

%%%
\section{Benchmark results}\label{appendix:results}
%%%

%
\subsection{Results analysis}

Note that performance is evaluated using the external index ARI (w.r.t. the ground-truth), while Stadion also uses $s$ = ARI as its similarity measure to estimate stability. It would be reasonable to expect this situation to introduce some kind of bias. However, results are not biased in favor of Stadion, as shown by Tables~(\ref{tab:ranking-km}, \ref{tab:ranking-ward}, \ref{tab:ranking-gmm}). Indeed, the ranking almost never changed while using different external indices to evaluate performance of Stadion, and keeping $s$ = ARI.

\begingroup
\setlength{\tabcolsep}{3.8pt} % Default value: 6pt
\begin{table*}
\caption{Performance rankings of clustering validation methods, evaluated with 16 external indices w.r.t. the ground-truth partitions, over 73 data sets for $K$-means. Rankings are mostly unchanged.}
\label{tab:ranking-km}
\centering
\begin{tiny}
% [inline block 0: 9 envs, 52227 chars -> data_tex | \begin{tabular}{lrrrrrrrrrrrrrrr}     \toprule...]

\end{tiny}
\end{center}
\endgroup
\end{table*}
